# Supplementary material for: GAAMA 2.0: An Integrated System that Answers Boolean and Extractive Questions
Source: arXiv:2206.08441 source file (2022-06-21)
Supplement: Supplementary file 1 [file appendix.tex]

\section{Ethical considerations}

Our machine reading comprehension system extends an existing MRC system and integrates capabilities that have previously existed in isolation, even though they are new to our system.
It is unlikely that this integration increases the risk of misuse of these capabilities.
Providing evidence to support YES/NO answers further decreases the risk of misuse of the system's output.

The data used originates from Wikipedia and is publicly available. All content conforms to Wikipedia's policies\footnote{\url{https://en.wikipedia.org/wiki/Wikipedia:What_Wikipedia_is_not#:~:text=Wikipediaspolicies}} for both living persons, offensive content, and any other information that may need quality control. Further details about the data collection can be found in the \tydi{} \cite{clark-etal-2020-tydi}, BoolQ \cite{clark-etal-2019-boolq}, and BoolQ-X \cite{rosenthal2021answers} papers.
%Our models were trained with publicly available datasets \tydi{} and BoolQ-X.
%These datasets use the Wikipedia and publicly available query logs that are believed not to contain publicly identifiable information.

Our models are based on transformers, which are known to be energy-intensive. 
We discuss modeling considerations (adapters)  that can reduce the expense and energy-intensiveness of applications such as this by reducing the number of GPUs required.
\label{sec:appendix}
